# Supplementary material for: Magnetically tuned topological phase in graphene nanoribbon heterojunctions
Source: arXiv:2412.00859 source file (2024-12-01)
Supplement: Supplementary file 1 [file SupplemantalMaterials.pdf]

# Supplemental Materials for
# Magnetically tuned topological phase in graphene nanoribbon heterojuctions

Wei-Jian Li,[1] Da-Fei Sun,[1] Sheng Ju,[2,3,*] Ai-Lei He,[4,†] and Yuan Zhou[1,5,‡]

[1] *National Laboratory of Solid State Microstructures and Department of Physics, Nanjing University, Nanjing, 210093, Jiangsu, China.*

[2] *School of Optical and Electronic Information, Suzhou City University, Suzhou 215104, China*

[3] *Jiangsu Key Laboratory and Suzhou Key Laboratory of Biophotonics, Suzhou City University, Suzhou 215104, China*

[4] *College of Physics Science and Technology, Yangzhou University, Yangzhou 225002, China*

[5] *Collaborative Innovation Center of Advanced Microstructures, Nanjing University, Nanjing, 210093, Jiangsu, China.*

(Dated: December 1, 2024)

## AB-INITIO CALCULATIONS

We study electronic and magnetic properties of the GNRH by the first-principle simulations. The first-principles simulation is performed in the framework of the density function theory implemented in the Quantum Espresso package [1]. We adopt the Perdew-Burke-Ernzerhof type generalized gradient approximation (GGA) [2] by using scalar relativistic and norm-conserving pseudopotentials of carbon and hydrogen with plane-wave cutoff of 90 Ry [3]. $k$-point grids are taken as ($\Gamma$ centered) $5 \times 1 \times 1$. Vacuum layer with 15 Å thickness is used in $x$- and $z$-direction to ensure the decoupling between neighboring slabs and zigzag shaped edges on both sides passivated by hydrogen atoms. In GGA, the electron-electron correlations is included via a mean-field-level approximation. To include electronic correlations beyond the GGA, we also used the GW approximations to calculate the quasiparticle bandstructure, as implemented in BerkeleyGW package [4]. The cut-off energy of dielectric function evaluation is 20 Ry and 2000 unoccupied bands (10 times of the valence bands) are used in the evaluation of dielectric function and the GW self-energy. We show the total energy of these configurations in Tab. S1. The limited energy difference, which is lower than 0.5 meV per carbon atom, makes those magnetic configurations highly tunable by external fields.

The bandgap of the NM configuration is about 17 meV (GGA) (Fig. S1 and Tab. S1), suggesting a narrow gap semiconductor. In contrast, the bandgap enhances about an order of magnitude in all magnetic configurations. In this sense, the introducing magnetism in GNRH may significantly improve the stability of potential topology. On the other hand, the magnitudes of bandgap under GW approximation is greatly enhanced about $4 - 9$ times. Similar enhancement of electron-electron interaction is widely observed in both AGNRs and ZGNRs [5, 6].

| Config. | NM | AFMA | AFMB | AFMC |
|---|---|---|---|---|
| Symm. | M/I | None | I | M |
| E | -9.707258 | -9.708250 | -9.707929 | -9.707702 |
| Gap (GGA) | 0.017 | 0.42 | 0.2 | 0.181 |
| Gap (GW) | 0.158 | 1.50 | 1.03 | 1.00 |

TABLE S1. Symmetry, total energy, and bandgap of respective configuration of the 2-3-9-17-GNRH. Here, "M", and "I" denotes the mirror, and inversion symmetry, respectively. The energy is averaged to each carbon atom, accurate to six decimal places. The two lower rows show bandgap obtained from the first-principle simulation with the GGA and GW methods. All energies are in unit of eV.

## MEAN-FIELD THEORY

We further simulate the magnetic and topological features of GNRHs by the $\pi$-orbital Hubbard model. The single $\pi$-orbital Hubbard model, which is capable of describing the low-energy physics of graphene, is described by the following Hamiltonian,

$$H = -t \sum_{<i,j>,\sigma} c^{\dagger}_{i\sigma} c_{j\sigma} + U \sum_{i} n_{i\uparrow} n_{i\downarrow}. \tag{1}$$

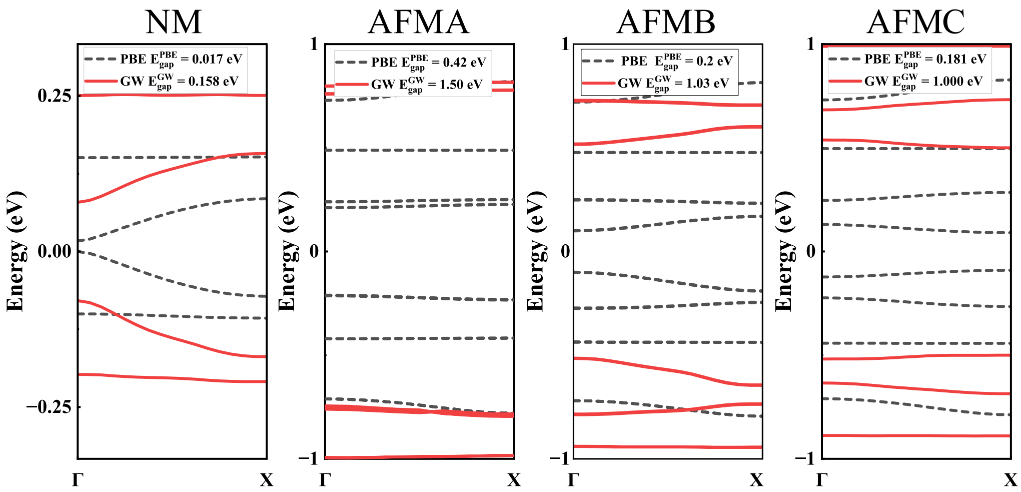


FIG. S1. Bandstructure of 2-3-9-17-GNRH in different magnetic configurations. The black dash lines, and the red solid lines are for the GGA (PBE), and GW approximation, respectively. The Fermi energy is fixed at zero.

Here $c_{i\sigma}$ is the electron annihilation operator with spin index $\sigma = \pm 1$ at site $i$ and $n_{i\sigma} = c^{\dagger}_{i\sigma} c_{i\sigma}$ is the electron number operator. For simplicity, we only consider the nearest neighboring hopping process with $t = 2.7$ eV. The effective on-site Coulomb repulsion $U$ is fixed at $1.0t$ [7, 8]. In fact, the main magnetic and topological properties are insensitive to the selected parameters. It was pointed out that the presence of long-range hopping processes dost not significantly affect the topological properties in GNR systems as revealed by the previous first-principle simulations [9].

## EVALUATION OF TOPOLOGICAL INDEX

### Junction index

For AGNRs with spatial symmetries, the $\Delta\mathbb{Z}_2$ invariant (0 or 1), defined by the difference of $\mathbb{Z}_2$ in respective AGNR, is applicable as suggested by Cao *et al.* in 7−9-GNRH [10]. However, the $\mathbb{Z}_2$ topological class in present heterojunctions is inadequate to characterize the $N_2 - N_1 > 2$ cases since it cannot figure out the difference between $\Delta\mathbb{Z}_2$ and $\Delta\mathbb{Z}_2 + 2m$ ($m$ is an integer). In our designed heterojunctions, the chiral symmetry ($A$ and $B$ sublattice symmetry) inherited from the original graphene honeycomb lattice is preserved, we therefore adopt the $\Delta\mathbb{Z}$ to characterize the topological index of the junction states. The $\mathbb{Z}$ index for arbitrary AGNR with commensurate unit cell and $\Delta\mathbb{Z}$ are defined as

$$\mathbb{Z} = N_{notco} - \lfloor \frac{N}{3} \rfloor,$$
$$\Delta\mathbb{Z} = \lfloor \frac{N_2}{3} \rfloor - \lfloor \frac{N_1}{3} \rfloor. \quad (2)$$

Here $N$ is the width of the AGNR, and $N_{notco}$ is the number of rows of atoms with carbon pairs not connected by $\sigma$-bonds within the specific unitcell that is commensurate to an anticipated termination [9]. The floor function $\lfloor a \rfloor$ denotes taking the largest integer less than or equal to the value $a$. $N_1$ and $N_2$ are the widths of left and right AGNR segments.

### Bulk index

If the unitcell of 1D crystal has the inversion or mirror symmetry, the SPT phase can be characterized by the $\mathbb{Z}_2$ invariant, determined by the product of the eigenvalues of inversion $\hat{I}$ or mirror $\hat{M}$ operator of the states at all the time reversal invariant momentum (TRIM) $k$ points in the occupied band manifold:

$$(-1)^{\mathbb{Z}_2} = \prod_{n \in occ} \prod_{\Gamma_{TRIM}} \langle \psi_{n\Gamma_{TRIM}} | \hat{O} | \psi_{n\Gamma_{TRIM}} \rangle, \quad (3)$$

where the operator $\hat{O}$ is the mirror operator $\hat{M}$ or inversion operator $\hat{I}$. The $\mathbb{Z}_2$ invariant can also be determined by calculating intercell Zak phase with the origin of the unitcell coinciding with the inversion or mirror center:[10, 11]:

$$\gamma_n = i2\pi \int_{-\pi}^{\pi} dk \langle \phi_{nk} | \nabla_k | \phi_{nk} \rangle$$
$$(-1)^{\mathbb{Z}_2} = e^{i \sum_n \gamma_n}. \tag{4}$$

The two methods are equivalent in the system with the inversion symmetry.

## SPIN-POLARIZED JUNCTION STATES

In main text, we show the typical topological junction states of 8-8-9-17 GNRH in NM and AFMB configurations with $\Delta\mathbb{Z} = 2$. Here, we further show the junction state of 8-8-9-13 GNRH but with $\Delta\mathbb{Z} = 1$ in Fig. S2. Here, only one junction state exists due to the relatively narrow ribbon and the nanoribbon is paramagnetic since $N_2 - N_1 = 4$The junction state locates on $A$ sublattice on left junction, while on $B$ sublattice on right junction, manifesting its chiral nature.

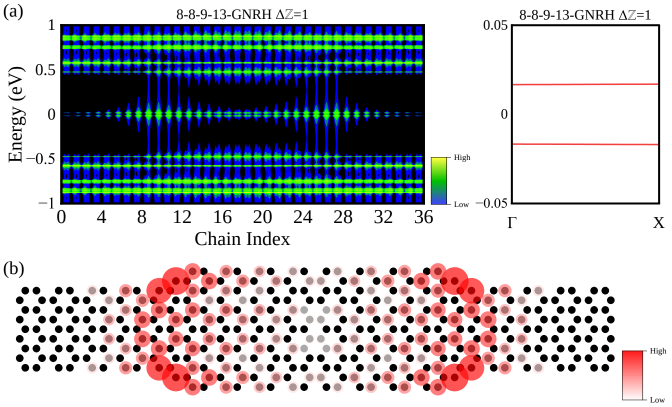


FIG. S2. Energy spectrum and real-space LDOS distribution of 8-8-11-13-GNRH. (a) Left: LDOS and energy spectrum map, the horizontal axis is the real-axis coordinate along $x$, the longitudinal axis is energy and the brightness stands for the relative strength of DOS. There is one degenerate state near the Fermi energy, as shown in the bandstructure in the right part. (b) The real-space resolved LDOS of the junction state.

We further show the similar junction states of 8-8-11-19 GNRH but with $\Delta\mathbb{Z} = 3$ in Fig. S3. The number and chirality of the junction state are independent of the emergent magnetism. Moreover, the bandgap in the magnetic configurations is much larger than that in the NM configurations, supporting the enhanced robustness of topological junction state in the magnetic configurations.

## EFFECTIVE SSH PARAMETERS

To model the topological phase transition in GNRHs, we calculate the maximally localized Wannier functions for the pair of conduction and valence bands closest to the Fermi level by the first-principle simulations. We then fit the conduction and valence band using the SSH model with the effective intra- and inter-dimer hopping $t_1$ and $t_2$ as shown in Table S2. The relative ratio of $|\frac{t_1}{t_2}|$ changes from $> 1$ to $< 1$ upon the selected geometries. The evolution of the intra- and inter-dimer hopping is well consistent with the topological phase diagram, supporting the SSH mechanism in present GNRHs.

* jusheng@suda.edu.cn
† heailei@yzu.edu.cn

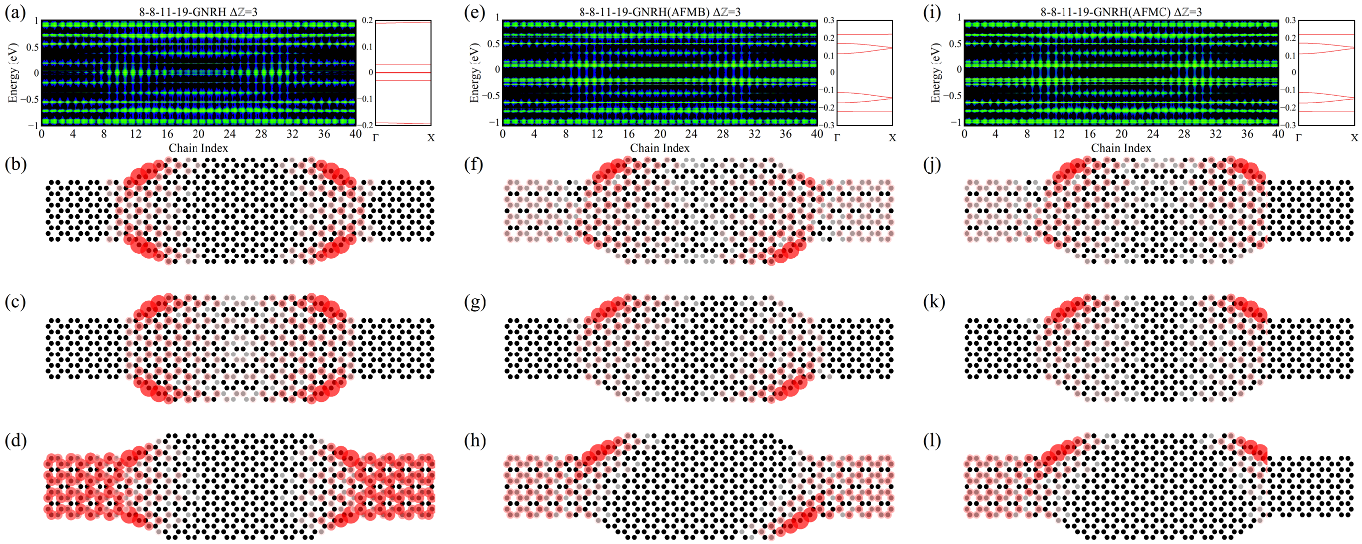


FIG. S3. Energy spectrum and real-space LDOS distribution of 8-8-11-19-GNRH. From left to right panels are NM, AFMB and AFMC configurations, respectively. Top panels are for the LDOS and energy spectrum map, the horizontal axis is the real-axis coordinate along $x$, the longitudinal axis is energy and the brightness stands for the relative strength of DOS. There is one nearly degenerate state near the Fermi energy in the NM configuration as shown in the bandstructure at the right of the LDOS map. Bottom panels are the real-space resolved LDOS of the junction state. For magnetic configurations, only one spin channel is shown.

| | AFMB | | AFMC | | NM | |
|---|---|---|---|---|---|---|
| | $t_1$ | $t_2$ | $t_1$ | $t_2$ | $t_1$ | $t_2$ |
| 2-3-5-13 | 86.317 | 1.702 | 56.462 | -16.958 | 46.013 | 1.8 |
| 2-3-7-15 | 46.478 | -124.12 | 118.71 | 139.45 | 67.354 | -6.664 |
| 2-3-9-17 | 11.324 | -142.18 | -3.695 | 114.47 | -35.095 | 6.705 |
| 2-8-9-17 | -4.446 | 162.61 | 0.11 | 28.506 | -0.966 | 6.697 |
| 8-2-9-17 | -1.753 | 130.23 | -2.147 | 58.173 | -70.103 | 0.02 |

TABLE S2. Hopping parameters (in unit of meV) between the Wannier centers of different configurations for several selected geometries. All data are direct obtained from the first-principle simulations

‡ zhouyuan@nju.edu.cn

[1] P. Giannozzi, S. Baroni, N. Bonini, M. Calandra, R. Car, C. Cavazzoni, D. Ceresoli, G. L. Chiarotti, M. Cococcioni, I. Dabo, A. D. Corso, S. de Gironcoli, S. Fabris, G. Fratesi, R. Gebauer, U. Gerstmann, C. Gougoussis, A. Kokalj, M. Lazzeri, L. Martin-Samos, N. Marzari, F. Mauri, R. Mazzarello, S. Paolini, A. Pasquarello, L. Paulatto, C. Sbraccia, S. Scandolo, G. Sclauzero, A. P. Seitsonen, A. Smogunov, P. Umari, and R. M. Wentzcovitch, Quantum espresso: a modular and open-source software project for quantum simulations of materials, J. Phys. Condens. Matter **21**, 395502 (2009).
[2] P. E. Blöchl, Projector augmented-wave method, Phys. Rev. B **50**, 17953 (1994).
[3] M. van Setten, M. Giantomassi, E. Bousquet, M. Verstraete, D. Hamann, X. Gonze, and G.-M. Rignanese, The pseudodojo: Training and grading a 85 element optimized norm-conserving pseudopotential table, Comput. Phys. Commun. **226**, 39 (2018).
[4] J. Deslippe, G. Samsonidze, D. A. Strubbe, M. Jain, M. L. Cohen, and S. G. Louie, Berkeleygw: A massively parallel computer package for the calculation of the quasiparticle and optical properties of materials and nanostructures, Comput. Phys. Commun. **183**, 1269 (2012).
[5] L. Yang, C. H. Park, Y. W. Son, M. L. Cohen, and S. G. Louie, Quasiparticle energies and band gaps in graphene nanoribbons, Phys. Rev. Lett. **99**, 186801 (2007).
[6] H. Hadipour, E. Şaşıoğlu, F. Bagherpour, C. Friedrich, S. Blügel, and I. Mertig, Screening of long-range coulomb interaction in graphene nanoribbons: Armchair versus zigzag edges, Phys. Rev. B **98**, 205123 (2018).
[7] A. Yamashiro, Y. Shimoi, K. Harigaya, and K. Wakabayashi, Spin- and charge-polarized states in nanographene ribbons with zigzag edges, Phys. Rev. B **68**, 193410 (2003).
[8] O. V. Yazyev, Magnetism in disordered graphene and irradiated graphite, Phys. Rev. Lett. **101**, 037203 (2008).
[9] J. Jiang and S. G. Louie, Topology classification using chiral symmetry and spin correlations in graphene nanoribbons, Nano. Lett. **21**, 197 (2021).

[10] T. Cao, F. Zhao, and S. G. Louie, Topological phases in graphene nanoribbons: Junction states, spin centers, and quantum spin chains, Phys. Rev. Lett. **119**, 076401 (2017).
[11] J.-W. Rhim, J. Behrends, and J. H. Bardarson, Bulk-boundary correspondence from the intercellular zak phase, Phys. Rev. B **95**, 035421 (2017).
